# Supplementary material for: Pipeline Interventions
Source: arXiv:2002.06592 source file (2020-08-28)
Supplement: Supplementary file 1 [file appendix_hardness.tex]

% \subsection{The Reduction}

% Our reduction works as follows: we construct a pipeline intervention instance of constant width (17 layers) from the given graph. The first layer has a node corresponding to each edge $(u,v)$ of the original graph, and is connected by edges to nodes corresponding to vertices $u$ and $v$ on the second layer. We set up the instance so that positive probability mass is only ever added to a set of edge disjoint paths, where each path corresponds to a vertex in the original graph. These paths are shown by the dark, solid lines in Figure~\ref{fig:hardness_instance}. The main idea behind the reduction is the following - by observing how allocations finding the maximin value split the budget over these edge disjoint paths, we can find out which vertices would form a small vertex cover of the original graph. 

% \begin{figure}[h]
%     \centering
%     \includegraphics[width=10cm]{hardness2.png}
%     \caption{Constructed Instance of the Pipeline Intervention problem}
%     \label{fig:hardness_instance}
% \end{figure}

% Formally, let the given graph $\cG=(\cV,\cE)$ we reduce from have $n$ vertices ($|\cV| =n $) and $m$ edges ($|\cE| = m$).  We construct of a pipeline intervention problem instance $\cI'$ with $k+2$ layers and width $w$, where $k =15$ and $w$ is polynomial in $n$. The instance $\cI'$ has an associated budget $B(\kappa, \varepsilon) = 2 k\kappa \varepsilon$ where $\varepsilon < \frac{1}{2}$. For the sake of clarity, we refer to the set of vertices $\cV$ in the vertex cover instance as ``vertices'' and the vertices in the instance $\cI'$ as ``nodes''. A complete description of instance $\cI'$ is as follows:
% \begin{enumerate}
%      \item The first layer, $L_1$, has exactly $m$ nodes, with each edge $(u,v)$ in graph $\cG$ having a unique corresponding node of the same label in layer $L_1$. 
%     \item The second layer has exactly $n$ nodes, with each vertex $v$ in graph $\cG$, having a unique corresponding node in layer $L_2$ with label $v^2$.
%     \item The next $k-1$ layers are of the following form - layer $L_i$, for $i=3$ to $k+1$, has $n+ 1$ nodes. The first $n$ nodes have labels from the set $\{v^i\}_{v \in V}$, i..e, each vertex $v$ in the original graph $\cG$ has a corresponding node $v^i$ in layer $L_i$. The last node is indexed by $x^i$ and exists to capture the ``leftover'' outward probability from the nodes $\{v^{i-1}\}_{v \in  V}$ in layer $L_{i-1}$.
%     \item The final layer $L_{k+2}$ has two reward nodes - $y$, of reward $1$ and $z$, of reward $0$. 
% \end{enumerate}  
% We now describe the initial transition matrices.
% \begin{enumerate}
%     \item From layer $L_1$ to layer $L_2$: for every node $(u,v)$ in layer $L_1$, the outgoing probability is equally split between edges to nodes $u^1$ and $v^1$ in layer $L_2$, i.e., edges $((u,v),u^1)$ and $((u,v),v^1)$ each have probability $\frac{1}{2}$.
%      \item From layer $L_i$ to layer $L_{i+1}$ for $i=2$ to $k$: For all vertices $v \in \cV$ (i.e., the original graph), the corresponding edge $(v^i,v^{i+1})$ (in our construction) has probability $\varepsilon$. The remaining outgoing probability out of node $v^i$ goes to the leakage node $x^{i+1}$. We call edges of the form $(v^i, x^{i+1})$ ``leakage'' edges. For $i \geq 3$, the edge $(x^i,x^{i+1})$ has all the outward probability, i.e., $1$,  from node $x^i$.
%     \item From layer $L_{k+1}$ to layer $L_{k+2}$: each node in layer $L_{k+1}$ is connected to $z$, the zero reward node, with probability $1$.
% \end{enumerate}

% We let $P_v$ be the path going through nodes $v^2,v^3 \cdots v^{k+1}, y$ in our construction. We will refer to $\{P_v\}_{v \in \cV}$ as vertex paths. Let $E'$ be the set of edges found on paths $\{P_v\}_{v \in V}$. Let $E''$ contain of all the ``leakage'' edges in the instance $\cI'$ ,i.e., edges of the form $(v^i, x^{i+1})$ as well as all edges of the form $(v^{k+1},z)$. We stipulate, as part of the description of the instance, that $E' \cup E''$ is the set of malleable edges in $\cI'$ and that the probability mass on any other edge cannot be changed. This completes the description of instance $\cI'$.


% \subsection{Proof of Hardness of Approximation}

% In this setup, we argue that any algorithm computing a maximin value of our instance will only use budget to improve the probability mass on the vertex paths. To begin, we observe that the only nodes with more than one outgoing malleable edge are the nodes on the vertex paths, exempting the reward node $y$. Hence, these are the only nodes whose associated outgoing transition matrices can be modified. Furthermore, these nodes have exactly one edge from $E'$, the edges on the vertex paths, and one leakage edge, implying that probability mass can only be transferred between these two edges. Note that the reward associated with starting at any leakage node is always $0$, since all outgoing edges from leakage nodes lead to the zero sink with probability $1$, and are not malleable.  
%  %and no other outgoing edges are present in the malleable edge set $E' \cup E''$. 
%  In contrast, nodes on the vertex paths start with expected positive welfare initially. Therefore, it would be a (strictly) sub-optimal strategy to route any more probability mass towards a leakage node , i.e., increase the probability mass on any edge in $E''$ leading to reward $0$, since it would come at the cost of decreasing probability mass on an edge towards a node on a vertex path with strictly positive reward. Consequently, any algorithm that optimizes the maximin value would only increase the probability on the other malleable edges, i.e., edges in $E'$, by removing probability mass from edges $E''$. To give a more local picture, budget is spent on the following operation - increasing the probability mass on an edge of the form $(v^i,v^{i+1})$ and balancing the outgoing probability mass from vertex $v^i$ by correspondingly decreasing the probability mass on edge $(v^i,x^{i+1})$. Note that there are no malleable edges in the transition between layer $L_1$ and layer $L_2$, and hence the corresponding transition matrix remains unchanged.

% We fix a threshold $T \triangleq \frac{(2 \varepsilon)^k}{4} $. The following lemma shows the desired reduction:
% \begin{lemma}
% \label{lemma:keyreduction}
% If graph $\cG$ has a vertex cover of size $\kappa$, then the maximin value of the constructed instance is at least $2T$. Complementarily, if graph $\cG$ has no vertex cover smaller than $1.3605 \kappa$, then the maximin value of the constructed instance is less than $T$.
% \end{lemma}
% Observe that the above lemma shows achieving a $2$-approximation to the maximin value is $\nph$-hard, since such an algorithm would be able to solve the gap version of vertex cover in polynomial time. Note that this also rules out an additive PTAS for the pipeline interventions problem, even for networks of constant depth , since our hard instance $\cI'$ has constant depth.

% %\proof{Proof of Lemma~\ref{lemma:keyreduction}}
% The forward direction of the proof is straightforward. Given that the original graph has a vertex cover $\cV^* \subseteq \cV$ of size $\kappa$, we show a candidate solution that guarantees a minimum reward of $2T$. Consider the subset $E^* \subseteq E$ which consists only of edges on the vertex paths indexed by vertices in the vertex cover $\cV^*$, i.e., $\{P_v\}_{v \in \cV^*}$. Since each such path has $k$ edges and there are $\kappa$ number of paths, $|E^*| = k \kappa$.
% We spend a budget $2 \varepsilon$ to increase the probability mass one each edge of $E^*$ by $\varepsilon$ and decrease the probability mass of the corresponding leakage edge by $\varepsilon$. Note that this is always possible, since $\varepsilon + \varepsilon \le 1$ (i.e., we never try to increase the probability mass on an edge beyond $1$). This exactly utilizes our budget $B(\kappa, \varepsilon) = 2k \kappa \varepsilon$. The new probability on every edge of $E^*$ is now $2\varepsilon$. Consider any population starting on a node $(u,v)$ of the first layer. Since $\cV^*$ is a vertex cover, at least one of $u$ or $v$ is present in the set $\cV^*$. Without loss of generality, let us assume $v \in \cV^*$. The reward at node $v^2$ is now exactly $(2\varepsilon)^k$. Since the transition matrices for layer $L_1$ to $L_2$ are unchanged, a population starting at node $(u,v)$ arrives at node $v^2$ with probability $\frac{1}{2}$; thus, an agent starting at $(u,v)$ has expected reward at least $\frac{(2 \varepsilon)^k}{2} = 2T$.

% Now, consider the case where the graph has no vertex cover of size $1.305 \kappa$. To prove a contradiction, let us assume that the maximin value is greater than or equal to $T$. We will show that we can recover a vertex cover of size less than size $1.305 \kappa$ from the maximin value solution, thus proving a contradiction. Let $W(l)$ represent the reward associated with starting at node $l$. We know that all the budget is spent on the paths $\{P_v\}_{v \in V}$. Let use write $2k \varepsilon a_v$ be the budget spent on improving path $P_v$; note that the net increase in probability mass across all edges of $P_v$ is $k \varepsilon a_v$. By the AM-GM inequality, we know that $W(v^2) \le (\varepsilon + a_v \varepsilon)^k$, with equality when $k a_v \varepsilon$ is split equally across edges on path $P_v$. A population starting at node $(u,v)$ on layer $L_1$ reaches node $u_2$ and node $v^2$ each with probability $\frac{1}{2}$ each. Thus, we have $W((u,v)) \le \frac{(\varepsilon + a_u \varepsilon)^k + (\varepsilon + a_v \varepsilon)^k}{2}$. Since this solution guarantees a reward of at least $T$ for every vertex within a total budget $B(\kappa, \varepsilon) = 2 k \kappa \varepsilon$, we have the following inequalities:
% \begin{align*}
%     \frac{(\varepsilon + a_u \varepsilon)^k + (\varepsilon + a_v \varepsilon)^k}{2} &\ge \frac{(2\varepsilon)^k}{4} \quad \forall (u,v) \in E
%     \\ \sum_{v \in V} a_v \le \kappa \varepsilon
% \end{align*}
% Dividing the first inequality by $\varepsilon^k$, multiplying by $2$, and substituting $k =15$, we get:
% \begin{align*}
%  (1 + a_u)^{15} + (1 + a_v)^{15} &\ge 2^{14} \quad \forall (u,v) \in E
%     \\ \sum_{v \in V} a_v \le \kappa
% \end{align*}
% We now generate a vertex set $\cV^*$ of original graph $\cG$ as follows - include vertex $v$ in $\cV^*$ if $a_v \ge 0.823$. We complete the proof by showing that $\cV^*$ is a vertex cover of $G$ and $|\cV^*| < 1.3605 \kappa$. The fact that $|\cV^*| < 1.3605 \kappa $ follows directly from the rounding scheme that is employed. Observe that each $a_v$ is scaled upward by a factor of at most $\frac{1}{0.823} < 1.22$. Thus, $|\cV^*| < 1.22 \kappa$. Now, assume that $\cV^*$ is not a vertex cover. Then, there exists an edge $(u,v) \in \cE$ in the original graph such that $a_u, a_v < 0.823$. Thus, we get:
% \begin{align*}
%     (1 + a_u)^{15} + (1 + a_v)^{15} &< 2 (1.823)^{15} < 16325< 16384 =   2^{14}
% \end{align*}
% This violates the reward guarantee for the population starting at node $(u,v)$, thus resulting in a contradiction.
% %\Halmos\endproof
